# Supplementary material for: Application of the ASBM-SA closure in a turbulent flow over a hump in the presence of separation control
Source: arXiv:2003.00579 source file (2020-03-01)
Supplement: Supplementary file 1 [file APPENDIX.tex]

\section{Details regarding the calibration process.}\label{appendix} 

The model coefficients of the proposed algebraic closures are determined based on the LES data
of Kaltenbach et al. \cite{kaltenbach1994}, who investigated the turbulent transport of three 
passive species which have uniform gradients in either the normal, streamwise or spanwise direction.
All cases under consideration start from the same  shear parameter ratio 
$S^{*}_{o} = \bigg( \frac{ 2 S \kappa}{\epsilon} \bigg)_{o} = 5.04$ and the same Prandtl number $Pr=1.0$, in the initial absent of scalar
fluctuations. The mean flow configuration is expressed by
\begin{equation}
G_{ij} = S\delta_{i1}\delta_{j3}\,,\qquad \Lambda_{i} = \Lambda \delta_{i\alpha}\,,
\end{equation}
where greek index $\alpha$ denotes the direction of the mean scalar gradient. 
\begin{table}[h!]
\centering
\begin{tabular}{c c c c c c c c c c}
\hline
$St$     &  $R_{11}$   &  $R_{13}$  &   $R_{22}$   &   $R_{33}$  & $\epsilon$  &    $\Lambda_{i}$       &  $\overline{ u'_{1}\phi' } $  &  $ \overline{ u'_{2}\phi' } $   &   $ \overline{ u'_{3}\phi' } $      \\ \hline
8 		 &  4.98       &   -1.42    &    2.82      &    1.60     &  0.911      &  $( 1,0,0 )$		&  -10.9          			    &                  		          &       2.22       				    \\
10 		 &  6.32       &   -1.84    &    3.63      &    2.20     &  1.190      &  $( 1,0,0 )$		&  -13.9          			    &                  				  &       3.01           				\\
12 		 &  7.67       &   -2.27    &    4.71      &    3.12     &  1.600      &  $( 1,0,0 )$		&  -16.3          			    &                  			      &       4.08          				 \\
8 		 &  4.98       &   -1.42    &    2.82      &    1.60     &  0.911      &  $( 0,1,0 )$		&                 			    &     -3.84        				  &                      				\\
10 		 &  6.32       &   -1.84    &    3.63      &    2.20     &  1.190      &  $( 0,1,0 )$		&                 			    &     -4.62        				  &                     				 \\
12 		 &  7.67       &   -2.27    &    4.71      &    3.12     &  1.600      &  $( 0,1,0 )$		&                 			    &     -5.78        				  &                     				 \\         
8 		 &  4.98       &   -1.42    &    2.82      &    1.60     &  0.911      &  $( 0,0,1 )$		&    4.32         			    &                  				  &       -1.83          				\\
10 		 &  6.32       &   -1.84    &    3.63      &    2.20     &  1.190      &  $( 0,0,1 )$		&    5.42         			    &                 				  &       -2.47         				\\
12 		 &  7.67       &   -2.27    &    4.71      &    3.12     &  1.600      &  $( 0,0,1 )$		&    6.33         			    &                  				  &       -3.42         				 \\  \hline     
\end{tabular}
\caption{ Summary of the LES data used to determine model coefficients. Data are extracted 
at different total shear instants $St$ (where $t$ is time). }
\label{table:calibration_data}
\end{table}
\FloatBarrier
